# Supplementary material for: Testing holography using lattice super-Yang--Mills on a 2-torus
Source: arXiv:1709.07025 ancillary file (2018-03-26)
Supplement: Supplementary file 1 [file tables.pdf]

## Testing holography using lattice super-Yang–Mills on a 2-torus

## — Supplemental tables —

In Tables S1–S16 we record the main results for the ensembles that appear in the body of the paper, specifically the Wilson loops $P_\beta$ and $P_L$ as well as the bosonic action density $-\langle s_{\text{Bos}}\rangle/(N^2\lambda)$. For the skewed torus with $\gamma = -1/2$ the last quantity is defined by

$$-\frac{s_{\text{Bos}}}{N^2\lambda} = \frac{27(1-s_B)(N^2-1)}{N^2\lambda_{\text{lat}}} \tag{S.1}$$

where $s_B = S_B/(N_x N_t(N^2-1))$ is normalized by the lattice size $N_x N_t$ and the number of SU($N$) generators $N^2-1$. (See the main text for the details of the relation between the continuum 't Hooft coupling and the lattice coupling $\lambda_{\text{lat}}$.) All results are obtained through blocked jackknife analyses with 100 molecular dynamics time units (MDTU) per block. For each ensemble we list the number of thermalized blocks.

Each ensemble is defined by $N$, the lattice size $N_x \times N_t$, the coupling $\lambda_{\text{lat}}$, and the two soft supersymmetry breaking parameters $\mu$ and $c_W$ described in the main text. Recalling $r_{\beta,\,\text{lat}} = N_t\sqrt{\lambda_{\text{lat}}}$ and $r_{L,\,\text{lat}} = N_x\sqrt{\lambda_{\text{lat}}}$, we organize the ensembles in terms of the aspect ratio $\alpha = r_L/r_\beta$ and the dimensionless temperature $t = 1/r_\beta = \sqrt[4]{27}/r_{\beta,\,\text{lat}}$. We also set $\mu$ so as to keep fixed the combination $\zeta \equiv \mu N_t/r_{\beta,\,\text{lat}}$ as we approach the $N_t \to \infty$ continuum limit. For aspect ratios $4 \le \alpha \le 8$ we only consider a single value of $\zeta^2 = 0.01$ with $c_W = 0$, which allows us to combine all SU($N$) gauge groups into a single table for each $\alpha$. For $1/2 \le \alpha \le 2$ we consider at least three values of $\zeta^2$ (with $c_W = \mu$) and linearly extrapolate $\zeta^2 \to 0$, setting up a separate table for each $N$.

| $t$ | $N$ | Blocks | $P_\beta$ | $P_L$ | $-\langle s_{\text{Bos}}\rangle/(N^2\lambda)$ |
|---|---|---|---|---|---|
| 13.4 | 6 | 20 | 0.994 108(53) | 0.344(12) | 62(6) |
| | 9 | 20 | 0.994 112(26) | 0.2496(90) | 58(4) |
| | 12 | 20 | 0.994 049(15) | 0.2043(72) | 55(2) |
| 14.2 | 6 | 20 | 0.994 493(39) | 0.415(11) | 66(4) |
| | 9 | 20 | 0.994 465(22) | 0.337(16) | 65(3) |
| | 12 | 20 | 0.994 419(17) | 0.352(15) | 63(2) |
| 15.2 | 6 | 20 | 0.994 871(31) | 0.5032(86) | 79(4) |
| | 9 | 20 | 0.994 851(23) | 0.475(13) | 73(5) |
| | 12 | 25 | 0.994 764(15) | 0.5030(62) | 78(2) |
| 16.3 | 6 | 20 | 0.995 242(27) | 0.5644(75) | 85(6) |
| | 9 | 25 | 0.995 175(19) | 0.5931(44) | 88(5) |
| | 12 | 25 | 0.995 133(14) | 0.5993(21) | 94(4) |
| 19.0 | 6 | 20 | 0.995 946(29) | 0.6897(35) | 121(9) |
| | 9 | 20 | 0.995 893(13) | 0.6906(20) | 122(7) |
| | 12 | 20 | 0.995 867(13) | 0.6890(10) | 124(4) |
| 22.8 | 6 | 20 | 0.996 693(21) | 0.7601(25) | 175(15) |
| | 9 | 20 | 0.996 639(15) | 0.7584(12) | 170(8) |
| | 12 | 20 | 0.996 599(14) | 0.7577(10) | 175(9) |

**Table S1**. Main results for SU(6), SU(9) and SU(12) $32\times4$ ensembles (aspect ratio $\alpha = 8$), with fixed $\zeta^2 = 0.01$ and $c_W = 0$. For this lattice size the SU(12) spatial deconfinement transition is located at $t_c = 14(1)$.

| $t$ | $N$ | Blocks | $P_\beta$ | $P_L$ | $-\langle s_{\text{Bos}}\rangle/(N^2\lambda)$ |
|---|---|---|---|---|---|
| 5.07 | 6 | 20 | 0.978 738(92) | 0.1748(26) | 12.9(8) |
| | 9 | 20 | 0.978 626(49) | 0.1167(14) | 13.2(4) |
| | 12 | 20 | 0.978 553(48) | 0.0877(10) | 13.7(3) |
| 5.7 | 6 | 20 | 0.981 938(75) | 0.1905(35) | 15.2(7) |
| | 9 | 20 | 0.981 806(59) | 0.1282(17) | 16.6(6) |
| | 12 | 20 | 0.981 601(34) | 0.0919(12) | 16.4(3) |
| 6.51 | 6 | 20 | 0.984 846(55) | 0.2121(44) | 19(1) |
| | 9 | 20 | 0.984 702(43) | 0.1399(25) | 19(1) |
| | 12 | 20 | 0.984 561(29) | 0.1057(22) | 20(1) |
| 7.6 | 6 | 20 | 0.987 591(92) | 0.2696(68) | 26(2) |
| | 9 | 20 | 0.987 536(35) | 0.1841(61) | 25(1) |
| | 12 | 20 | 0.987 454(36) | 0.1386(31) | 24(1) |
| 8.29 | 6 | 20 | 0.988 83(12) | 0.326(11) | 24(2) |
| | 9 | 20 | 0.988 841(38) | 0.2324(69) | 27(1) |
| | 12 | 20 | 0.988 773(24) | 0.1819(56) | 28(1) |
| 9.12 | 6 | 20 | 0.990 092(97) | 0.431(11) | 33(2) |
| | 9 | 20 | 0.989 925(41) | 0.368(12) | 36(2) |
| | 12 | 20 | 0.989 880(23) | 0.372(15) | 35(1) |
| 10.13 | 6 | 20 | 0.991 176(64) | 0.5626(80) | 41(3) |
| | 9 | 20 | 0.990 967(47) | 0.5689(49) | 42(2) |
| | 12 | 20 | 0.990 955(25) | 0.5728(25) | 46(2) |
| 11.4 | 6 | 20 | 0.992 081(88) | 0.6383(58) | 49(4) |
| | 9 | 20 | 0.992 006(32) | 0.6562(13) | 57(3) |
| | 12 | 20 | 0.992 026(20) | 0.6595(13) | 57(2) |
| 13.03 | 6 | 20 | 0.993 261(62) | 0.7184(33) | 64(7) |
| | 9 | 20 | 0.993 126(24) | 0.7185(14) | 71(3) |
| | 12 | 20 | 0.993 092(16) | 0.7177(14) | 71(3) |

**Table S2**. Main results for SU(6), SU(9) and SU(12) $24\times4$ ensembles (aspect ratio $\alpha = 6$), with fixed $\zeta^2 = 0.01$ and $c_W = 0$. For this lattice size the SU(12) spatial deconfinement transition is located at $t_c = 9(1)$.

| $t$ | $N$ | Blocks | $P_\beta$ | $P_L$ | $-\langle s_{\rm Bos}\rangle/(N^2\lambda)$ |
|---|---|---|---|---|---|
| 3.8 | 6 | 20 | 0.968 41(14) | 0.2555(68) | 7.3(6) |
| | 9 | 20 | 0.968 38(19) | 0.1685(60) | 8.5(8) |
| | 12 | 20 | 0.968 08(7) | 0.1380(28) | 8.3(4) |
| 4.14 | 6 | 20 | 0.971 81(16) | 0.2876(92) | 10.0(8) |
| | 9 | 20 | 0.971 88(9) | 0.2185(55) | 9.5(6) |
| | 12 | 20 | 0.971 66(7) | 0.1673(66) | 9.9(5) |
| 4.34 | 6 | 20 | 0.973 29(13) | 0.328(10) | 9.4(8) |
| | 9 | 20 | 0.973 00(17) | 0.251(14) | 10.7(8) |
| | 12 | 20 | 0.973 13(6) | 0.2036(66) | 10.3(5) |
| 4.56 | 6 | 20 | 0.974 97(11) | 0.3793(92) | 13(1) |
| | 9 | 20 | 0.974 58(11) | 0.308(11) | 11(1) |
| | 12 | 20 | 0.974 67(6) | 0.314(13) | 11(1) |
| 4.8 | 6 | 20 | 0.976 37(10) | 0.4497(98) | 12(1) |
| | 9 | 20 | 0.976 11(9) | 0.397(16) | 13(1) |
| | 12 | 20 | 0.975 96(8) | 0.425(17) | 13(1) |
| 5.07 | 6 | 20 | 0.977 65(11) | 0.4991(58) | 14(1) |
| | 9 | 20 | 0.977 51(7) | 0.509(11) | 13(1) |
| | 12 | 20 | 0.977 30(5) | 0.5436(46) | 16(1) |
| 5.7 | 6 | 20 | 0.980 66(15) | 0.6203(73) | 16(2) |
| | 9 | 20 | 0.980 11(7) | 0.6313(28) | 20(1) |
| | 12 | 20 | 0.980 21(6) | 0.6310(14) | 19(1) |
| 6.51 | 6 | 20 | 0.982 90(16) | 0.6934(40) | 25(2) |
| | 9 | 20 | 0.982 98(6) | 0.6948(18) | 28(1) |
| | 12 | 20 | 0.982 89(4) | 0.6939(12) | 26(1) |
| 7.6 | 6 | 20 | 0.985 94(13) | 0.7467(27) | 31(4) |
| | 9 | 20 | 0.985 59(6) | 0.7507(11) | 34(2) |
| | 12 | 20 | 0.985 52(4) | 0.7481(15) | 38(2) |

**Table S3**. Main results for SU(6), SU(9) and SU(12) $24\times6$ ensembles (aspect ratio $\alpha = 4$), with fixed $\zeta^2 = 0.01$ and $c_W = 0$. For this lattice size the SU(12) spatial deconfinement transition is located at $t_c = 4.6(2)$.

| $t$ | $N$ | Blocks | $P_\beta$ | $P_L$ | $-\langle s_{\text{Bos}}\rangle/(N^2\lambda)$ |
|---|---|---|---|---|---|
| 3.8 | 6 | 20 | 0.968 97(16) | 0.2641(63) | 8.47(41) |
| | 9 | 20 | 0.9688(1) | 0.1705(36) | 8.80(22) |
| | 12 | 20 | 0.968 63(9) | 0.1311(45) | 8.61(23) |
| 4.14 | 6 | 35 | 0.9722(1) | 0.3078(49) | 10.46(37) |
| | 9 | 20 | 0.9722(1) | 0.2164(61) | 9.52(44) |
| | 12 | 35 | 0.971 99(5) | 0.1686(30) | 9.98(20) |
| 4.34 | 6 | 20 | 0.973 66(15) | 0.3436(88) | 9.94(58) |
| | 9 | 20 | 0.9737(1) | 0.2580(56) | 10.28(42) |
| | 12 | 20 | 0.973 54(8) | 0.2143(87) | 10.58(30) |
| 4.56 | 6 | 35 | 0.9753(1) | 0.3840(76) | 12.19(41) |
| | 9 | 20 | 0.9750(1) | 0.349(12) | 12.20(68) |
| | 12 | 27 | 0.975 12(7) | 0.316(10) | 12.02(28) |
| 4.8 | 6 | 20 | 0.976 57(9) | 0.4477(92) | 13.82(46) |
| | 9 | 20 | 0.9762(1) | 0.4501(82) | 13.10(65) |
| | 12 | 20 | 0.976 21(7) | 0.455(12) | 13.51(36) |
| 5.07 | 6 | 35 | 0.9781(1) | 0.4982(78) | 15.31(71) |
| | 9 | 20 | 0.9777(1) | 0.5367(57) | 14.87(54) |
| | 12 | 27 | 0.977 61(6) | 0.5310(75) | 14.94(45) |
| 5.7 | 6 | 35 | 0.9808(1) | 0.6106(39) | 17.84(88) |
| | 9 | 20 | 0.9805(1) | 0.6349(16) | 18.94(83) |
| | 12 | 30 | 0.980 27(4) | 0.6301(12) | 18.90(52) |
| 6.51 | 6 | 35 | 0.9835(1) | 0.6879(22) | 25.1(13) |
| | 9 | 20 | 0.9830(1) | 0.6910(21) | 26.5(12) |
| | 12 | 20 | 0.983 08(4) | 0.6936(13) | 25.75(66) |

**Table S4**. Main results for SU(6), SU(9) and SU(12) $16\times4$ ensembles (aspect ratio $\alpha = 4$), with fixed $\zeta^2 = 0.01$ and $c_W = 0$. For this lattice size the SU(12) spatial deconfinement transition is located at $t_c = 4.6(2)$.

| $t$ | $N$ | Blocks | $P_\beta$ | $P_L$ | $-\langle s_{\text{Bos}}\rangle/(N^2\lambda)$ |
|---|---|---|---|---|---|
| 4.56 | 9 | 20 | 0.955 03(23) | 0.9499(2) | 39.7(4) |
| | 12 | 20 | 0.955 09(12) | 0.9498(1) | 43.6(3) |
| 5.07 | 9 | 20 | 0.959 74(29) | 0.9560(3) | 53.9(7) |
| | 12 | 20 | 0.959 76(12) | 0.9555(1) | 56.5(4) |
| 5.7 | 9 | 20 | 0.964 38(18) | 0.9607(2) | 62(1) |
| | 12 | 20 | 0.964 19(12) | 0.9609(1) | 63(1) |
| 6.5 | 9 | 20 | 0.969 04(12) | 0.9662(1) | 84(1) |
| | 12 | 20 | 0.968 70(10) | 0.9665(1) | 94(1) |
| 7.6 | 9 | 20 | 0.973 46(17) | 0.9714(1) | 119(2) |
| | 12 | 20 | 0.973 11(11) | 0.9712(1) | 127(1) |
| 9.1 | 9 | 20 | 0.977 49(15) | 0.9763(1) | 165(2) |
| | 12 | 20 | 0.977 61(6) | 0.9762(1) | 183(1) |

**Table S5**. Main results for high-temperature SU(9) and SU(12) 8×8 ensembles (aspect ratio $\alpha = 1$), with fixed $\zeta^2 = 0.01$ and $c_W = 0$.

| $t$ | $\zeta^2$ | Blocks | $P_\beta$ | $P_L$ | $-\langle s_{\text{Bos}}\rangle/(N^2\lambda)$ |
|---|---|---|---|---|---|
| 0.33 | 0.04 | 20 | 0.231(13) | 0.817(22) | 0.351(11) |
| | 0.02 | 20 | 0.3166(76) | 0.681(11) | 0.213(7) |
| | 0.01 | 20 | 0.3353(67) | 0.709(13) | 0.146(7) |
| | $\longrightarrow 0$ | $\chi^2$/d.o.f. = 0.01/1, CL = 0.93 | | | 0.077(9) |
| 0.38 | 0.04 | 20 | 0.3665(69) | 0.694(12) | 0.433(12) |
| | 0.02 | 20 | 0.398(11) | 0.735(16) | 0.257(12) |
| | 0.01 | 20 | 0.4284(54) | 0.712(8) | 0.195(11) |
| | $\longrightarrow 0$ | $\chi^2$/d.o.f. = 1.56/1, CL = 0.21 | | | 0.108(14) |
| 0.46 | 0.04 | 20 | 0.4788(51) | 0.816(11) | 0.464(12) |
| | 0.02 | 20 | 0.459(10) | 0.933(18) | 0.285(14) |
| | 0.01 | 20 | 0.5046(73) | 0.887(25) | 0.215(14) |
| | $\longrightarrow 0$ | $\chi^2$/d.o.f. = 0.51/1, CL = 0.48 | | | 0.125(17) |
| 0.52 | 0.04 | 20 | 0.5509(56) | 0.0859(17) | 0.531(26) |
| | 0.02 | 20 | 0.552(13) | 0.1015(20) | 0.326(26) |
| | 0.01 | 20 | 0.5845(50) | 0.0888(21) | 0.285(23) |
| | $\longrightarrow 0$ | $\chi^2$/d.o.f. = 1.77/1, CL = 0.18 | | | 0.187(29) |
| 0.57 | 0.04 | 20 | 0.5916(64) | 0.909(13) | 0.561(31) |
| | 0.02 | 20 | 0.5630(80) | 0.1111(26) | 0.370(28) |
| | 0.01 | 20 | 0.5741(81) | 0.1093(19) | 0.276(25) |
| | $\longrightarrow 0$ | $\chi^2$/d.o.f. = 0.0005/1, CL = 0.98 | | | 0.180(32) |
| 0.64 | 0.04 | 20 | 0.6165(66) | 0.0968(20) | 0.641(38) |
| | 0.02 | 20 | 0.599(13) | 0.1158(20) | 0.417(29) |
| | 0.01 | 20 | 0.6444(64) | 0.0997(15) | 0.341(29) |
| | $\longrightarrow 0$ | $\chi^2$/d.o.f. = 0.41/1, CL = 0.52 | | | 0.231(38) |
| 0.69 | 0.04 | 20 | 0.6618(67) | 0.1052(23) | 0.651(40) |
| | 0.02 | 20 | 0.613(11) | 0.1258(26) | 0.447(45) |
| | 0.01 | 20 | 0.6408(68) | 0.1246(31) | 0.408(38) |
| | $\longrightarrow 0$ | $\chi^2$/d.o.f. = 0.63/1, CL = 0.43 | | | 0.311(48) |

**Table S6**. Main results for SU(12) 24×12 ensembles (aspect ratio $\alpha = 2$), with $c_W = \mu$.

| $t$ | $\zeta^2$ | Blocks | $P_\beta$ | $P_L$ | $-\langle s_{\text{Bos}}\rangle/(N^2\lambda)$ |
|---|---|---|---|---|---|
| 0.33 | 0.04 | 15 | 0.2864(41) | 0.0312(8) | 0.375(6) |
| | 0.02 | 20 | 0.3456(13) | 0.0305(6) | 0.217(3) |
| | 0.01 | 20 | 0.3835(34) | 0.0432(6) | 0.138(5) |
| | $\longrightarrow 0$ | $\chi^2$/d.o.f. = 0.0008/1, CL = 0.98 | | | 0.060(6) |
| 0.38 | 0.04 | 25 | 0.4047(11) | 0.0349(5) | 0.404(5) |
| | 0.02 | 20 | 0.4354(10) | 0.0358(6) | 0.242(6) |
| | 0.01 | 20 | 0.4710(32) | 0.0494(8) | 0.163(5) |
| | $\longrightarrow 0$ | $\chi^2$/d.o.f. = 0.03/1, CL = 0.87 | | | 0.082(6) |
| 0.46 | 0.04 | 15 | 0.474(12) | 0.0639(14) | 0.428(10) |
| | 0.02 | 20 | 0.485(12) | 0.0737(12) | 0.257(7) |
| | 0.01 | 20 | 0.5498(41) | 0.0786(14) | 0.192(7) |
| | $\longrightarrow 0$ | $\chi^2$/d.o.f. = 2.47/1, CL = 0.12 | | | 0.109(9) |
| 0.52 | 0.04 | 20 | 0.5864(8) | 0.0459(7) | 0.509(12) |
| | 0.02 | 25 | 0.5980(5) | 0.0464(8) | 0.342(8) |
| | 0.01 | 20 | 0.6085(36) | 0.0633(13) | 0.251(10) |
| | $\longrightarrow 0$ | $\chi^2$/d.o.f. = 0.20/1, CL = 0.65 | | | 0.168(12) |
| 0.57 | 0.04 | 22 | 0.6244(6) | 0.0498(12) | 0.541(15) |
| | 0.02 | 17 | 0.6330(4) | 0.0514(11) | 0.389(19) |
| | 0.01 | 20 | 0.6364(6) | 0.0507(9) | 0.268(12) |
| | $\longrightarrow 0$ | $\chi^2$/d.o.f. = 2.02/1, CL = 0.16 | | | 0.183(16) |
| 0.64 | 0.04 | 30 | 0.6731(5) | 0.0526(8) | 0.629(14) |
| | 0.02 | 19 | 0.6781(5) | 0.0543(9) | 0.442(23) |
| | 0.01 | 26 | 0.6819(5) | 0.0539(8) | 0.354(19) |
| | $\longrightarrow 0$ | $\chi^2$/d.o.f. = 0.03/1, CL = 0.87 | | | 0.261(23) |
| 0.69 | 0.04 | 24 | 0.7022(4) | 0.0582(9) | 0.662(17) |
| | 0.02 | 25 | 0.7070(4) | 0.0610(12) | 0.480(20) |
| | 0.01 | 22 | 0.7105(4) | 0.0605(12) | 0.374(18) |
| | $\longrightarrow 0$ | $\chi^2$/d.o.f. = 0.17/1, CL = 0.68 | | | 0.283(22) |

**Table S7**. Main results for SU(16) 16×8 ensembles (aspect ratio $\alpha = 2$), with $c_W = \mu$.

| $t$ | $\zeta^2$ | Blocks | $P_\beta$ | $P_L$ | $-\langle s_{\text{Bos}}\rangle/(N^2\lambda)$ |
|---|---|---|---|---|---|
| 0.33 | 0.04 | 20 | 0.245(10) | 0.0618(7) | 0.355(7) |
| | 0.02 | 20 | 0.3476(38) | 0.0545(9) | 0.230(5) |
| | 0.01 | 20 | 0.3826(38) | 0.0563(7) | 0.156(4) |
| | $\longrightarrow 0$ | $\chi^2$/d.o.f. = 1.64/1, CL = 0.20 | | | 0.092(6) |
| 0.38 | 0.04 | 20 | 0.3941(57) | 0.0650(11) | 0.389(8) |
| | 0.02 | 20 | 0.4197(49) | 0.0652(9) | 0.241(5) |
| | 0.01 | 20 | 0.4638(46) | 0.0679(9) | 0.173(6) |
| | $\longrightarrow 0$ | $\chi^2$/d.o.f. = 0.43/1, CL = 0.51 | | | 0.098(8) |
| 0.46 | 0.04 | 20 | 0.4803(52) | 0.0749(9) | 0.454(10) |
| | 0.02 | 20 | 0.5228(41) | 0.0696(23) | 0.269(8) |
| | 0.01 | 20 | 0.5489(36) | 0.0783(12) | 0.221(9) |
| | $\longrightarrow 0$ | $\chi^2$/d.o.f. = 7.60/1, CL = 0.01 | | | 0.126(11) |
| 0.52 | 0.04 | 20 | 0.5579(50) | 0.0848(18) | 0.504(13) |
| | 0.02 | 20 | 0.5972(8) | 0.0635(12) | 0.354(17) |
| | 0.01 | 20 | 0.5975(44) | 0.0867(14) | 0.249(9) |
| | $\longrightarrow 0$ | $\chi^2$/d.o.f. = 1.14/1, CL = 0.29 | | | 0.167(13) |
| 0.57 | 0.04 | 20 | 0.5934(57) | 0.0900(12) | 0.541(19) |
| | 0.02 | 20 | 0.6246(55) | 0.0910(18) | 0.352(13) |
| | 0.01 | 20 | 0.6377(6) | 0.0676(10) | 0.318(14) |
| | $\longrightarrow 0$ | $\chi^2$/d.o.f. = 5.54/1, CL = 0.02 | | | 0.224(18) |
| 0.64 | 0.04 | 20 | 0.6570(51) | 0.0798(23) | 0.617(22) |
| | 0.02 | 20 | 0.6789(5) | 0.0742(12) | 0.447(17) |
| | 0.01 | 20 | 0.6701(52) | 0.0970(16) | 0.377(19) |
| | $\longrightarrow 0$ | $\chi^2$/d.o.f. = 0.18/1, CL = 0.67 | | | 0.291(24) |
| 0.69 | 0.04 | 20 | 0.7023(8) | 0.0766(13) | 0.698(29) |
| | 0.02 | 20 | 0.7074(5) | 0.0786(11) | 0.528(20) |
| | 0.01 | 20 | 0.6928(35) | 0.1023(16) | 0.411(17) |
| | $\longrightarrow 0$ | $\chi^2$/d.o.f. = 0.74/1, CL = 0.39 | | | 0.320(24) |

**Table S8**. Main results for SU(12) 16×8 ensembles (aspect ratio $\alpha = 2$), with $c_W = \mu$.

| $t$ | $\zeta^2$ | Blocks | $P_\beta$ | $P_L$ | $-\langle s_{\text{Bos}}\rangle/(N^2\lambda)$ |
|---|---|---|---|---|---|
| 0.28 | 0.04 | 20 | 0.1669(67) | 0.1576(59) | 0.315(10) |
| | 0.02 | 20 | 0.1715(54) | 0.1739(71) | 0.177(12) |
| | 0.01 | 40 | 0.1813(33) | 0.1717(39) | 0.109(7) |
| | $\longrightarrow 0$ | $\chi^2$/d.o.f. = 0.00004/1, CL = 0.99 | | | 0.040(10) |
| 0.33 | 0.04 | 20 | 0.1897(69) | 0.1927(58) | 0.351(17) |
| | 0.02 | 20 | 0.2075(89) | 0.1929(59) | 0.208(17) |
| | 0.01 | 40 | 0.1931(43) | 0.1949(40) | 0.136(9) |
| | $\longrightarrow 0$ | $\chi^2$/d.o.f. = 0.0018/1, CL = 0.97 | | | 0.064(14) |
| 0.38 | 0.04 | 44 | 0.2284(69) | 0.2121(63) | 0.371(16) |
| | 0.02 | 50 | 0.2418(74) | 0.2199(60) | 0.315(13) |
| | 0.03 | 50 | 0.2117(46) | 0.2093(52) | 0.208(15) |
| | 0.01 | 50 | 0.2091(48) | 0.2152(48) | 0.141(13) |
| | $\longrightarrow 0$ | $\chi^2$/d.o.f. = 2.32/2, CL = 0.31 | | | 0.060(17) |
| 0.46 | 0.04 | 40 | 0.4241(40) | 0.3565(40) | 0.577(23) |
| | 0.03 | 40 | 0.4326(42) | 0.3674(29) | 0.457(21) |
| | 0.02 | 40 | 0.3297(81) | 0.3096(93) | 0.309(19) |
| | 0.01 | 40 | 0.288(10) | 0.2711(91) | 0.204(17) |
| | $\longrightarrow 0$ | $\chi^2$/d.o.f. = 0.88/2, CL = 0.65 | | | 0.072(22) |
| 0.52 | 0.04 | 40 | 0.4884(38) | 0.4223(36) | 0.626(33) |
| | 0.02 | 40 | 0.393(20) | 0.359(15) | 0.328(29) |
| | 0.01 | 40 | 0.4178(87) | 0.3680(61) | 0.257(27) |
| | $\longrightarrow 0$ | $\chi^2$/d.o.f. = 2.11/1, CL = 0.15 | | | 0.112(35) |
| 0.57 | 0.04 | 20 | 0.5331(62) | 0.4665(61) | 0.765(53) |
| | 0.02 | 20 | 0.460(29) | 0.363(25) | 0.360(53) |
| | 0.01 | 20 | 0.432(23) | 0.407(25) | 0.340(37) |
| | $\longrightarrow 0$ | $\chi^2$/d.o.f. = 3.96/1, CL = 0.05 | | | 0.169(51) |
| 0.64 | 0.04 | 20 | 0.5698(56) | 0.5097(52) | 0.724(61) |
| | 0.02 | 20 | 0.383(24) | 0.359(19) | 0.451(59) |
| | 0.01 | 20 | 0.463(28) | 0.447(26) | 0.501(57) |
| | $\longrightarrow 0$ | $\chi^2$/d.o.f. = 2.93/1, CL = 0.09 | | | 0.368(71) |

**Table S9**. Main results for SU(12) 16×16 ensembles (aspect ratio $\alpha = 1$), with $c_W = \mu$.

| $t$ | $\zeta^2$ | Blocks | $P_\beta$ | $P_L$ | $-\langle s_{\text{Bos}}\rangle/(N^2\lambda)$ |
|---|---|---|---|---|---|
| 0.28 | 0.04 | 20 | 0.1915(42) | 0.2086(72) | 0.368(20) |
| | 0.02 | 20 | 0.1915(82) | 0.1998(86) | 0.229(14) |
| | 0.01 | 20 | 0.2027(59) | 0.2000(56) | 0.152(15) |
| | $\longrightarrow 0$ | $\chi^2$/d.o.f. = 0.08/1, CL = 0.77 | | | 0.082(19) |
| 0.33 | 0.04 | 20 | 0.2066(65) | 0.2098(73) | 0.384(19) |
| | 0.02 | 20 | 0.220(13) | 0.2091(66) | 0.247(22) |
| | 0.01 | 20 | 0.2304(76) | 0.2219(80) | 0.142(18) |
| | $\longrightarrow 0$ | $\chi^2$/d.o.f. = 0.89/1, CL = 0.34 | | | 0.070(22) |
| 0.38 | 0.04 | 20 | 0.2473(98) | 0.2378(82) | 0.381(33) |
| | 0.02 | 20 | 0.2424(97) | 0.2265(65) | 0.249(40) |
| | 0.01 | 20 | 0.2474(72) | 0.2329(70) | 0.164(30) |
| | $\longrightarrow 0$ | $\chi^2$/d.o.f. = 0.07/1, CL = 0.79 | | | 0.096(39) |
| 0.46 | 0.04 | 20 | 0.2842(83) | 0.2639(98) | 0.430(49) |
| | 0.02 | 20 | 0.267(11) | 0.2588(94) | 0.357(51) |
| | 0.01 | 20 | 0.2517(88) | 0.2731(83) | 0.221(43) |
| | $\longrightarrow 0$ | $\chi^2$/d.o.f. = 1.18/1, CL = 0.28 | | | 0.177(35) |
| 0.52 | 0.04 | 20 | 0.330(12) | 0.3097(96) | 0.452(71) |
| | 0.02 | 20 | 0.281(14) | 0.275(11) | 0.318(51) |
| | 0.01 | 20 | 0.2781(73) | 0.2471(75) | 0.187(43) |
| | $\longrightarrow 0$ | $\chi^2$/d.o.f. = 0.45/1, CL = 0.50 | | | 0.111(60) |
| 0.57 | 0.04 | 20 | 0.379(15) | 0.361(13) | 0.570(59) |
| | 0.02 | 20 | 0.384(16) | 0.362(11) | 0.582(69) |
| | 0.01 | 20 | 0.287(13) | 0.294(13) | 0.243(63) |
| | $\longrightarrow 0$ | $\chi^2$/d.o.f. = 7.74/1, CL = 0.01 | | | 0.238(77) |
| 0.64 | 0.04 | 20 | 0.443(20) | 0.435(14) | 0.588(71) |
| | 0.02 | 20 | 0.375(21) | 0.376(22) | 0.51(10) |
| | 0.01 | 20 | 0.342(15) | 0.313(18) | 0.334(81) |
| | $\longrightarrow 0$ | $\chi^2$/d.o.f. = 0.61/1, CL = 0.44 | | | 0.28(10) |

**Table S10**. Main results for SU(9) 16×16 ensembles (aspect ratio $\alpha = 1$), with $c_W = \mu$.

| $t$ | $\zeta^2$ | Blocks | $P_\beta$ | $P_L$ | $-\langle s_{\text{Bos}}\rangle/(N^2\lambda)$ |
|---|---|---|---|---|---|
| 0.28 | 0.04 | 14 | 0.1335(77) | 0.1214(70) | 0.324(4) |
| | 0.02 | 40 | 0.2287(42) | 0.1398(36) | 0.199(3) |
| | 0.01 | 20 | 0.2576(18) | 0.1723(33) | 0.145(4) |
| | $\longrightarrow 0$ | $\chi^2$/d.o.f. = 1.85/1, CL = 0.17 | | | 0.081(5) |
| 0.33 | 0.04 | 18 | 0.221(13) | 0.1813(96) | 0.351(6) |
| | 0.02 | 14 | 0.3014(27) | 0.2094(38) | 0.236(6) |
| | 0.01 | 18 | 0.3333(18) | 0.2391(20) | 0.170(6) |
| | $\longrightarrow 0$ | $\chi^2$/d.o.f. = 0.71/1, CL = 0.40 | | | 0.113(7) |
| 0.38 | 0.04 | 22 | 0.3538(19) | 0.2488(32) | 0.424(7) |
| | 0.02 | 17 | 0.3927(22) | 0.2977(23) | 0.284(12) |
| | 0.01 | 12 | 0.4113(13) | 0.3231(22) | 0.185(9) |
| | $\longrightarrow 0$ | $\chi^2$/d.o.f. = 1.95/1, CL = 0.16 | | | 0.111(11) |
| 0.46 | 0.04 | 15 | 0.4641(18) | 0.3666(23) | 0.520(13) |
| | 0.02 | 15 | 0.4887(16) | 0.3961(19) | 0.363(14) |
| | 0.01 | 20 | 0.4981(10) | 0.4112(16) | 0.266(10) |
| | $\longrightarrow 0$ | $\chi^2$/d.o.f. = 0.58/1, CL = 0.45 | | | 0.184(13) |
| 0.52 | 0.04 | 26 | 0.5385(13) | 0.4519(13) | 0.612(15) |
| | 0.02 | 18 | 0.5547(14) | 0.4691(15) | 0.451(17) |
| | 0.01 | 20 | 0.5630(10) | 0.4825(13) | 0.330(13) |
| | $\longrightarrow 0$ | $\chi^2$/d.o.f. = 1.84/1, CL = 0.18 | | | 0.244(17) |
| 0.57 | 0.04 | 26 | 0.5775(11) | 0.5204(10) | 0.710(21) |
| | 0.02 | 14 | 0.5887(8) | 0.5119(18) | 0.521(23) |
| | 0.01 | 21 | 0.5971(7) | 0.4927(12) | 0.429(16) |
| | $\longrightarrow 0$ | $\chi^2$/d.o.f. = 0.01/1, CL = 0.94 | | | 0.335(21) |
| 0.64 | 0.04 | 16 | 0.6273(9) | 0.5486(15) | 0.771(28) |
| | 0.02 | 15 | 0.6368(13) | 0.5620(10) | 0.635(27) |
| | 0.01 | 21 | 0.6411(8) | 0.5682(9) | 0.504(18) |
| | $\longrightarrow 0$ | $\chi^2$/d.o.f. = 1.93/1, CL = 0.16 | | | 0.424(25) |
| 0.69 | 0.04 | 23 | 0.6582(6) | 0.5838(9) | 0.897(24) |
| | 0.02 | 20 | 0.6658(6) | 0.5967(9) | 0.707(20) |
| | 0.01 | 21 | 0.6710(7) | 0.6043(7) | 0.593(28) |
| | $\longrightarrow 0$ | $\chi^2$/d.o.f. = 0.19/1, CL = 0.66 | | | 0.501(31) |

**Table S11**. Main results for SU(16) 8×8 ensembles (aspect ratio $\alpha = 1$), with $c_W = \mu$.

| $t$ | $\zeta^2$ | Blocks | $P_\beta$ | $P_L$ | $-\langle s_{\text{Bos}}\rangle/(N^2\lambda)$ |
|---|---|---|---|---|---|
| 0.28 | 0.04 | 20 | 0.1397(56) | 0.1432(44) | 0.336(6) |
| | 0.02 | 20 | 0.1662(70) | 0.1436(48) | 0.195(6) |
| | 0.01 | 20 | 0.1696(65) | 0.1507(50) | 0.121(5) |
| | $\longrightarrow 0$ | $\chi^2$/d.o.f. = 0.14/1, CL = 0.70 | | | 0.050(6) |
| 0.33 | 0.04 | 20 | 0.1868(72) | 0.1752(58) | 0.347(7) |
| | 0.02 | 20 | 0.2716(83) | 0.1899(67) | 0.233(8) |
| | 0.01 | 20 | 0.3176(47) | 0.2311(35) | 0.175(7) |
| | $\longrightarrow 0$ | $\chi^2$/d.o.f. = 0.01/1, CL = 0.91 | | | 0.118(9) |
| 0.38 | 0.04 | 20 | 0.3123(83) | 0.2378(54) | 0.412(9) |
| | 0.02 | 20 | 0.3845(22) | 0.2886(40) | 0.283(9) |
| | 0.01 | 20 | 0.4116(33) | 0.3068(41) | 0.188(9) |
| | $\longrightarrow 0$ | $\chi^2$/d.o.f. = 3.37/1, CL = 0.07 | | | 0.123(11) |
| 0.46 | 0.04 | 20 | 0.4613(19) | 0.3610(22) | 0.517(16) |
| | 0.02 | 20 | 0.4850(16) | 0.3919(22) | 0.351(15) |
| | 0.01 | 20 | 0.4948(32) | 0.4007(33) | 0.288(9) |
| | $\longrightarrow 0$ | $\chi^2$/d.o.f. = 0.65/1, CL = 0.42 | | | 0.210(12) |
| 0.52 | 0.04 | 20 | 0.5354(17) | 0.4463(21) | 0.631(16) |
| | 0.02 | 20 | 0.5526(13) | 0.4625(20) | 0.447(17) |
| | 0.01 | 20 | 0.5603(13) | 0.4777(16) | 0.358(15) |
| | $\longrightarrow 0$ | $\chi^2$/d.o.f. = 0.01/1, CL = 0.91 | | | 0.266(19) |
| 0.57 | 0.04 | 20 | 0.5753(18) | 0.4878(26) | 0.656(19) |
| | 0.02 | 20 | 0.5913(13) | 0.5104(12) | 0.494(30) |
| | 0.01 | 20 | 0.5587(55) | 0.4551(44) | 0.352(16) |
| | $\longrightarrow 0$ | $\chi^2$/d.o.f. = 1.52/1, CL = 0.22 | | | 0.257(21) |
| 0.64 | 0.04 | 20 | 0.6248(9) | 0.5451(15) | 0.815(23) |
| | 0.02 | 20 | 0.6339(8) | 0.5585(18) | 0.572(28) |
| | 0.01 | 20 | 0.6337(30) | 0.5532(67) | 0.514(28) |
| | $\longrightarrow 0$ | $\chi^2$/d.o.f. = 1.49/1, CL = 0.22 | | | 0.391(33) |
| 0.69 | 0.04 | 20 | 0.6571(13) | 0.5792(14) | 0.893(27) |
| | 0.02 | 20 | 0.6647(11) | 0.5933(8) | 0.744(31) |
| | 0.01 | 20 | 0.6466(62) | 0.5784(50) | 0.586(29) |
| | $\longrightarrow 0$ | $\chi^2$/d.o.f. = 2.17/1, CL = 0.14 | | | 0.509(35) |

**Table S12**. Main results for SU(12) 8×8 ensembles (aspect ratio $\alpha = 1$), with $c_W = \mu$.

| $t$ | $\zeta^2$ | Blocks | $P_\beta$ | $P_L$ | $-\langle s_{\text{Bos}}\rangle/(N^2\lambda)$ |
|---|---|---|---|---|---|
| 0.25 | 0.04 | 30 | 0.1342(28) | 0.1627(63) | 0.334(10) |
| | 0.02 | 19 | 0.1393(30) | 0.1771(76) | 0.192(12) |
| | 0.01 | 20 | 0.1399(40) | 0.1674(72) | 0.102(7) |
| | $\longrightarrow 0$ | $\chi^2$/d.o.f. = 0.96/1, CL = 0.33 | | | 0.027(9) |
| 0.28 | 0.04 | 23 | 0.1465(27) | 0.1858(64) | 0.347(10) |
| | 0.02 | 23 | 0.1515(42) | 0.1920(94) | 0.209(13) |
| | 0.01 | 20 | 0.1514(39) | 0.202(11) | 0.133(13) |
| | $\longrightarrow 0$ | $\chi^2$/d.o.f. = 0.10/1, CL = 0.75 | | | 0.064(15) |
| 0.33 | 0.04 | 27 | 0.1596(39) | 0.2057(95) | 0.370(13) |
| | 0.02 | 40 | 0.1669(33) | 0.2027(88) | 0.217(11) |
| | 0.01 | 20 | 0.1731(56) | 0.191(12) | 0.164(12) |
| | $\longrightarrow 0$ | $\chi^2$/d.o.f. = 1.19/1, CL = 0.28 | | | 0.087(15) |
| 0.38 | 0.04 | 23 | 0.2220(90) | 0.373(17) | 0.467(16) |
| | 0.02 | 30 | 0.2845(40) | 0.464(10) | 0.337(22) |
| | 0.01 | 20 | 0.1852(54) | 0.189(14) | 0.161(23) |
| | $\longrightarrow 0$ | $\chi^2$/d.o.f. = 7.14/1, CL = 0.01 | | | 0.102(27) |
| 0.46 | 0.04 | 20 | 0.3318(62) | 0.538(15) | 0.575(35) |
| | 0.02 | 55 | 0.3505(67) | 0.550(13) | 0.392(21) |
| | 0.01 | 11 | 0.3875(81) | 0.606(12) | 0.256(31) |
| | $\longrightarrow 0$ | $\chi^2$/d.o.f. = 0.85/1, CL = 0.36 | | | 0.171(37) |

**Table S13**. Main results for SU(16) $8\times16$ ensembles (aspect ratio $\alpha = 1/2$), with $c_W = \mu$.

| $t$ | $\zeta^2$ | Blocks | $P_\beta$ | $P_L$ | $-\langle s_{\text{Bos}}\rangle/(N^2\lambda)$ |
|---|---|---|---|---|---|
| 0.25 | 0.04 | 20 | 0.1575(40) | 0.199(11) | 0.350(14) |
| | 0.02 | 20 | 0.1580(33) | 0.1983(95) | 0.199(8) |
| | 0.01 | 20 | 0.1631(47) | 0.195(11) | 0.118(15) |
| | $\longrightarrow 0$ | $\chi^2$/d.o.f. = 0.09/1, CL = 0.76 | | | 0.044(16) |
| 0.28 | 0.04 | 20 | 0.1758(39) | 0.218(13) | 0.341(16) |
| | 0.02 | 20 | 0.1765(47) | 0.1923(85) | 0.240(17) |
| | 0.01 | 20 | 0.1838(53) | 0.2089(96) | 0.144(15) |
| | $\longrightarrow 0$ | $\chi^2$/d.o.f. = 2.40/1, CL = 0.12 | | | 0.091(19) |
| 0.33 | 0.04 | 20 | 0.1886(39) | 0.2261(90) | 0.355(30) |
| | 0.02 | 20 | 0.1970(42) | 0.232(11) | 0.253(24) |
| | 0.01 | 20 | 0.1991(38) | 0.2246(96) | 0.157(15) |
| | $\longrightarrow 0$ | $\chi^2$/d.o.f. = 1.13/1, CL = 0.29 | | | 0.095(22) |
| 0.38 | 0.04 | 20 | 0.1963(37) | 0.224(12) | 0.424(32) |
| | 0.02 | 20 | 0.2067(53) | 0.2281(90) | 0.247(21) |
| | 0.01 | 20 | 0.2102(43) | 0.2347(91) | 0.204(26) |
| | $\longrightarrow 0$ | $\chi^2$/d.o.f. = 1.14/1, CL = 0.29 | | | 0.113(32) |
| 0.46 | 0.04 | 20 | 0.2957(67) | 0.438(19) | 0.541(52) |
| | 0.02 | 20 | 0.2258(47) | 0.2510(91) | 0.297(35) |
| | 0.01 | 20 | 0.2292(71) | 0.248(15) | 0.295(45) |
| | $\longrightarrow 0$ | $\chi^2$/d.o.f. = 2.64/1, CL = 0.10 | | | 0.164(55) |

**Table S14**. Main results for SU(12) $8\times16$ ensembles (aspect ratio $\alpha = 1/2$), with $c_W = \mu$.

| $t$ | $\zeta^2$ | Blocks | $P_\beta$ | $P_L$ | $-\langle s_{\text{Bos}}\rangle/(N^2\lambda)$ |
|---|---|---|---|---|---|
| 0.25 | 0.04 | 20 | 0.1490(21) | 0.1693(60) | 0.349(11) |
| | 0.02 | 20 | 0.1479(29) | 0.1965(79) | 0.207(8) |
| | 0.01 | 20 | 0.1672(45) | 0.204(10) | 0.138(11) |
| | $\longrightarrow 0$ | $\chi^2$/d.o.f. = 0.01/1, CL = 0.93 | | | 0.067(12) |
| 0.28 | 0.04 | 20 | 0.1661(36) | 0.217(13) | 0.366(12) |
| | 0.02 | 20 | 0.1686(29) | 0.2012(82) | 0.209(13) |
| | 0.01 | 20 | 0.1805(34) | 0.2201(98) | 0.137(14) |
| | $\longrightarrow 0$ | $\chi^2$/d.o.f. = 0.06/1, CL = 0.80 | | | 0.058(16) |
| 0.33 | 0.04 | 19 | 0.1822(39) | 0.2079(82) | 0.362(15) |
| | 0.02 | 20 | 0.1846(29) | 0.2128(53) | 0.224(16) |
| | 0.01 | 20 | 0.1910(43) | 0.221(13) | 0.178(15) |
| | $\longrightarrow 0$ | $\chi^2$/d.o.f. = 0.60/1, CL = 0.44 | | | 0.110(18) |
| 0.38 | 0.04 | 20 | 0.2030(50) | 0.241(12) | 0.400(17) |
| | 0.02 | 20 | 0.2012(52) | 0.2162(89) | 0.249(26) |
| | 0.01 | 20 | 0.2102(51) | 0.2182(96) | 0.182(24) |
| | $\longrightarrow 0$ | $\chi^2$/d.o.f. = 0.04/1, CL = 0.84 | | | 0.107(29) |
| 0.46 | 0.04 | 20 | 0.2438(88) | 0.309(20) | 0.463(25) |
| | 0.02 | 20 | 0.2291(51) | 0.2516(90) | 0.308(34) |
| | 0.01 | 20 | 0.2185(58) | 0.244(14) | 0.291(24) |
| | $\longrightarrow 0$ | $\chi^2$/d.o.f. = 1.10/1, CL = 0.29 | | | 0.221(31) |

**Table S15**. Main results for SU(12) $6\times12$ ensembles (aspect ratio $\alpha = 1/2$), with $c_W = \mu$.

| $t$ | $\zeta^2$ | Blocks | $P_\beta$ | $P_L$ | $-\langle s_{\text{Bos}}\rangle/(N^2\lambda)$ |
|---|---|---|---|---|---|
| 0.25 | 0.04 | 20 | 0.1868(46) | 0.2113(67) | 0.362(14) |
| | 0.02 | 20 | 0.1749(31) | 0.2205(89) | 0.301(16) |
| | 0.01 | 20 | 0.1793(39) | 0.229(12) | 0.218(12) |
| | $\longrightarrow 0$ | $\chi^2$/d.o.f. = 0.35/1, CL = 0.56 | | | 0.075(27) |
| 0.28 | 0.04 | 20 | 0.2021(32) | 0.2413(85) | 0.396(13) |
| | 0.02 | 20 | 0.1974(57) | 0.244(10) | 0.317(16) |
| | 0.01 | 20 | 0.1986(30) | 0.229(11) | 0.249(16) |
| | $\longrightarrow 0$ | $\chi^2$/d.o.f. = 0.09/1, CL = 0.76 | | | 0.100(33) |
| 0.33 | 0.04 | 20 | 0.2096(35) | 0.2373(99) | 0.424(18) |
| | 0.02 | 20 | 0.2118(49) | 0.2421(91) | 0.380(22) |
| | 0.01 | 20 | 0.2191(34) | 0.282(13) | 0.280(23) |
| | $\longrightarrow 0$ | $\chi^2$/d.o.f. = 1.16/1, CL = 0.28 | | | 0.151(47) |
| 0.38 | 0.04 | 20 | 0.2366(49) | 0.270(11) | 0.417(27) |
| | 0.02 | 20 | 0.2350(65) | 0.246(10) | 0.418(30) |
| | 0.01 | 20 | 0.2406(47) | 0.255(11) | 0.305(27) |
| | $\longrightarrow 0$ | $\chi^2$/d.o.f. = 2.63/1, CL = 0.11 | | | 0.209(59) |
| 0.46 | 0.04 | 20 | 0.2538(43) | 0.287(17) | 0.489(44) |
| | 0.02 | 20 | 0.2510(52) | 0.280(11) | 0.478(44) |
| | 0.01 | 20 | 0.2571(65) | 0.261(13) | 0.376(48) |
| | $\longrightarrow 0$ | $\chi^2$/d.o.f. = 0.69/1, CL = 0.41 | | | 0.28(10) |

**Table S16**. Main results for SU(9) $6\times12$ ensembles (aspect ratio $\alpha = 1/2$), with $c_W = \mu$.
